# Supplementary material for: Tests of Macrorealism in Discrete and Continuous Variable Systems
Source: arXiv:2402.16537 source file (2024-02-26)
Supplement: Supplementary file 1 [file appendices.tex]

\chapter{Appendices}
